# Supplementary material for: Cluster Expansion Toward Nonlinear Modeling and Classification
Source: arXiv:2506.18695 ancillary file (2025-06-23)
Supplement: Supplementary file 1 [file supplementary-material-prr.pdf]

# Supplemental Material for Cluster Expansion Toward Nonlinear Modeling and Classification

Adrian Stroth, Claudia Draxl, and Santiago Rigamonti*

*Physics Department and CSMB, Humboldt-Universität zu Berlin, 12489 Berlin, Germany*

## I. REDLICH-KISTER MODEL

The Redlich-Kister model of the Gibbs energy of alloys is defined in Eq. (5.21) of Ref. [1]. For the particular case of a binary alloy, composed of atomic species A and B, at zero temperature, it reads:

$$G(\boldsymbol{\sigma}) = x_A\, g_0 + x_B\, g_1 + J(x_B - x_A)\, x_A x_B, \tag{1}$$

with $J(y)$ representing a concentration-dependent interaction between nearest-neighbor (nn) A and B species, defined as

$$J(y) = \sum_{\nu=0}^{\nu_{\max}} \omega_\nu y^\nu, \tag{2}$$

with $x_B =: x$, and $x_A = 1 - x$ being their concentrations in the alloy. Typically, a value of $\nu_{\max} = 2$ is chosen, as also in the case here. In Eq. (1), the factor $x_A x_B$ originates from the limiting value of the concentration of nn AB bonds, $x_{AB}(\boldsymbol{\sigma})$, in the perfectly disordered alloy (see Section I C),

$$x_{AB}(\boldsymbol{\sigma}) \to 2x_A x_B = 2x(1-x). \tag{3}$$

In this work, we generalize Eq.(1) by replacing this limiting value by the actual concentration of AB bonds of configuration $\boldsymbol{\sigma}$:

$$G(\boldsymbol{\sigma}) = x_A\, g_0 + x_B\, g_1 + \frac{1}{2} J(x_B - x_A)\, x_{AB}(\boldsymbol{\sigma}). \tag{4}$$

This makes the expression for the Gibbs energy configuration dependent, in contrast to Eq. (1), which solely depends on $x$. Eq. (4) also retains the defininig feature of the Redlich-Kister Gibbs energy, namely, the nonlinear interaction between nn species A and B, while being identical to Eq. (1) in the perfectly disordered alloy limit.

### A. Synthetic data

In order to generate synthetic data for training a cluster expansion (CE) model, a binary two-dimensional square lattice with 64 lattice sites is considered. The energies of 132 random atomic configurations with concentrations $x \in [0, 1]$ are computed using Eq. (4) toghether with the parameters shown in Table I.

| $g_0$ | $g_1$ | $\omega_0$ | $\omega_1$ | $\omega_2$ |
|---|---|---|---|---|
| 0.8 | 1.0 | -1.0 | 5.0 | 1.0 |

Supplementary Table I. Coefficients of the Redlich-Kister model of Eq. (4).

The data used for training are shown by the black circles in Fig. 1. It can be seen that, for concentrations other than 0 or 1, there is a configuration dependence, *i.e.*, different configurations at the same concentration yield different energies.

We fit a standard CE model with a pool of 18 clusters containing up to nn three-body interactions and using a LASSO estimator. This yields a dense model with rather inaccurate predictions shown by the crosses in Fig. 1. On the other

* srigamonti@physik.hu-berlin.de

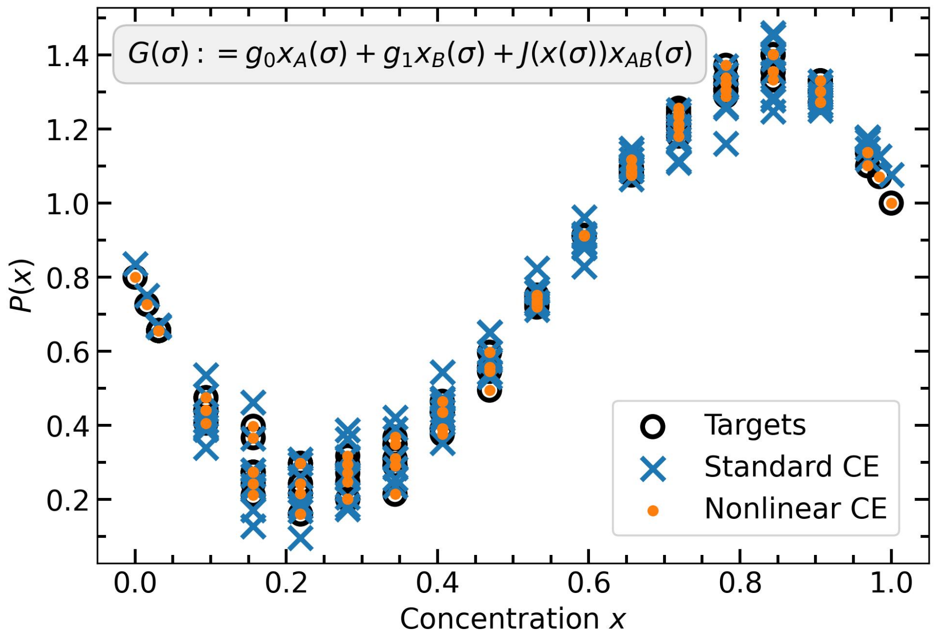


Supplementary Fig. 1. Predictions of standard (blue crosses) and nonlinear CE (orange dots) of the toy model $P(x)$ target values (black circles) as a function of the substituent concentration x.

hand, a nonlinear CE with 19 polynomial features up to degree 3 based on a smaller pool of clusters with up to second nn two-body interactions and a LASSO estimator, yields exact predictions shown by the orange dots in Fig. 1. In both cases, leave-one-out cross validation is used to determine the optimal hyperparameter $\lambda$. For the standard CE, a $\lambda$ value of $2.66\times10^{-5}$ is found, while for nonlinear CE, it is $1\times10^{-7}$.

All the CE modeling, including standard and nonlinear CE, was performed with the package `CELL`[2, 3].

### B. Cluster correlations

We employ a single-site cluster basis defined by

$$\begin{aligned}\phi_0(\sigma) &= 1,\\ \phi_1(\sigma) &= \sigma,\\ \sigma &= 0, 1,\end{aligned} \tag{5}$$

where $\sigma$ indicates the occupation of a crystal site, such that $\sigma = 0$ if the site is occupied with species A, and $\sigma = 1$ if the site is occupied with species B. The correlation of the 1-body cluster reads

$$X_{1b}(\boldsymbol{\sigma}) = \frac{1}{N}\sum_{i=1}^{N}\sigma_i =: \langle\sigma\rangle,$$

where $N$ is the number of crystal sites. Then the concentration $x$ is simply related to $X_{1b}(\boldsymbol{\sigma})$:

$$\begin{aligned}x &= \frac{1}{N}\sum_{i=1}^{N}\sigma_i\\ x &= X_{1b}(\boldsymbol{\sigma}).\end{aligned} \tag{6}$$

Now we look into the 2-point nn correlation

$$X_{2nn}(\boldsymbol{\sigma}) := \frac{1}{N_{2nn}}\sum_{\langle ij\rangle=1}^{N_{2nn}}\sigma_i\sigma_j, \tag{7}$$

| Term | Intercept | $X_{1b}$ | $X_{2nn}$ | $X_{1b}^2$ | $X_{1b}X_{2nn}$ | $X_{1b}^3$ | $X_{1b}^2X_{2nn}$ |
|---|---|---|---|---|---|---|---|
| Coefficient | $K_0$ | $K_1$ | $K_2$ | $K_3$ | $K_4$ | $K_5$ | $K_6$ |
| Value | 0.8 | -4.8 | 5.0 | 6.0 | -6.0 | 4.0 | -4.0 |
| log\|Value\| | -0.22 | -1.57 | 1.61 | 1.79 | -1.79 | 1.39 | -1.39 |
| Relation | $g_0$ | $g_1 - g_0 + \omega_0 - \omega_1 + \omega_2$ | $-\omega_0 + \omega_1 - \omega_2$ | $2\omega_1 - 4\omega_2$ | $-2\omega_1 + 4\omega_2$ | $4\omega_2$ | $-4\omega_2$ |

Supplementary Table II. Coefficients of the nonlinear CE and relationship to the Redlich-Kister model. The coefficients $K_{1..6}$ correspond to the feature indices 1, 2, 4, 5, 10, and 11 of Fig. 1 of the main paper.

where $N_{2nn}$ is the number of nn pairs of sites in the crystal. To see how this result relates to the concentration $x_{AB}(\boldsymbol{\sigma})$ of nn pairs AB, we compute the latter as follows:

$$\begin{aligned}
x_{AB}(\boldsymbol{\sigma}) &= \frac{1}{N_{2nn}} \sum_{\langle ij \rangle=1}^{N_{2nn}} [(1-\sigma_i)\sigma_j + \sigma_i(1-\sigma_j)] \\
&= \frac{1}{N_{2nn}} \sum_{\langle ij \rangle=1}^{N_{2nn}} [\sigma_j - \sigma_i\sigma_j + \sigma_i - \sigma_i\sigma_j] \\
&= 2\frac{1}{N_{2nn}} \sum_{\langle ij \rangle=1}^{N_{2nn}} \sigma_i - 2\frac{1}{N_{2nn}} \sum_{\langle ij \rangle=1}^{N_{2nn}} \sigma_i\sigma_j \\
&= 2X_{1b}(\boldsymbol{\sigma}) - 2X_{2nn}(\boldsymbol{\sigma}) \\
&= 2\left[X_{1b}(\boldsymbol{\sigma}) - X_{2nn}(\boldsymbol{\sigma})\right]. \qquad (8)
\end{aligned}$$

Note that we have used the obvious fact that $\sum_{\langle ij \rangle=1}^{N_{2nn}} \sigma_i/N_{2nn} = \sum_{\langle ij \rangle=1}^{N} \sigma_i/N$.

To write the Redlich-Kister model in terms of cluster correlations, we replace $x$ and $x_{AB}(\boldsymbol{\sigma})$ in Eqs. (4) by Eqs. (6) and (8), respectively. The result is:

$$\begin{aligned}
G(\boldsymbol{\sigma}) =& K_0 + K_1X_{1b}(\boldsymbol{\sigma}) + K_2X_{2nn}(\boldsymbol{\sigma}) + K_3X_{1b}(\boldsymbol{\sigma})^2 + K_4X_{1b}(\boldsymbol{\sigma})X_{2nn}(\boldsymbol{\sigma}) \qquad (9) \\
&+ K_5X_{1b}(\boldsymbol{\sigma})^3 + K_6X_{1b}(\boldsymbol{\sigma})^2X_{2nn}(\boldsymbol{\sigma})
\end{aligned}$$

with

$$\begin{aligned}
K_0 &= g_0 \\
K_1 &= g_1 - g_0 + \omega_0 - \omega_1 + \omega_2 \\
K_2 &= -\omega_0 + \omega_1 - \omega_2 \\
K_3 &= 2\omega_1 - 4\omega_2 \qquad (10) \\
K_4 &= -2\omega_1 + 4\omega_2 \\
K_5 &= 4\omega_2 \\
K_6 &= -4\omega_2 \,.
\end{aligned}$$

Table II shows the values of the coefficients $K_0 - K_6$ (see row "Value") as computed from Eq. (10) with the parameters of Table I. The row "log|Value|" shows the (signed) logarithm of the coefficients to facilitate the comparison with the coefficients $\mathcal{K}$ in Fig. 1 of the main paper, obtained by nonlinear CE with LASSO. The coefficients $K_1 - K_6$ correspond to the feature indices 1, 2, 4, 5, 10, and 11 of Fig. 1 of the main paper. The agreement of the nonlinear CE with the analytic solution derived here is remarkable, meaning that the nonlinear CE is able to recover the Redlich-Kister model exactly, while the standard CE does not.

### C. Perfectly disordered alloy

In this section, we prove Eq. (3). To this extent, we analyze Eq. (7) in the limit of the perfectly disordered alloy (d). In this case, the value of $X_{2nn}(\boldsymbol{\sigma})$ can be computed as

$$\begin{aligned} X_{2nn}^{(\mathrm{d})} &= \frac{1}{N_{2nn}} \sum_{\langle ij \rangle=1}^{N_{2nn}} \langle \sigma_i \sigma_j \rangle_{(\mathrm{d})} \\ &= \frac{1}{N_{2nn}} \sum_{\langle ij \rangle=1}^{N_{2nn}} \langle \sigma_i \rangle \langle \sigma_j \rangle \\ &= \frac{1}{N_{2nn}} \sum_{\langle ij \rangle=1}^{N_{2nn}} x^2 \\ X_{2nn}^{(\mathrm{d})} &= x^2. \end{aligned}$$

Here, we have used that $\langle \sigma_i \sigma_j \rangle = \langle \sigma_i \rangle \langle \sigma_j \rangle$ as required for a fully disordered system. Using this result, Eq. (6), and Eq. (8) we arrive, as expected, at the limiting expression for $x_{AB}$, namely

$$x_{AB}^{(d)} = 2(x - x^2) = 2x(1 - x) = 2x_A x_B.$$

## II. RELATION BETWEEN NONLINEAR CE AND A MODIFIED BAYESIAN CE

In Ref. [4], a method is proposed to extend the standard CE to model the energy-configuration relationship for nanoparticles. The method proposes the replacement of the constant term $J_0$, usually termed empty-cluster ECI, by a function of the number $n$ of substituent atoms, $J_{0,n}$. This extension can be expressed as follows:

$$P(\boldsymbol{\sigma}) = J_{0,n(\boldsymbol{\sigma})} + \sum_{i \neq 0} \mathcal{J}_i X_i(\boldsymbol{\sigma}) \tag{11}$$

Here, $X_i(\boldsymbol{\sigma}) = \langle \Gamma_{\boldsymbol{\alpha}_i}(\boldsymbol{\sigma}) \rangle$, as defined after Eq.(3) of the main manuscript, and $n(\boldsymbol{\sigma})$ is the number of substituent atoms in the nanoparticle with configuration $\boldsymbol{\sigma}$.

Since this method has been employed to account for significant composition-dependent effects, it is interesting to compare the CE originating from Eq. 11 with the method presented by us. However, before doing so, Eq. 11 must be adapted for solids. To this end, we propose to replace the function $J_{0,n}$, which depends on the discrete integer variable $n$, by a function $J_0(x)$ of the continuous variable $x$ belonging to the continuous real interval $[0, 1]$:

$$P(\boldsymbol{\sigma}) = J_0(x) + \sum_{i \neq 0} \mathcal{J}_i X_i(\boldsymbol{\sigma}) \tag{12}$$

To keep the description simple, we consider the case of a binary system using the basis of Eq.5. Such a basis is non-orthogonal, which is not relevant for this comparison, since an analogous result is obtained with an orthogonal basis. Using Eq.6 and assuming that there is only a single type of 1-point clusters indexed $i = 1$, then

$$X_1(\boldsymbol{\sigma}) = x \tag{13}$$

Thus, we get

$$P(\boldsymbol{\sigma}) = J_0(X_1(\boldsymbol{\sigma})) + \sum_{i \neq 0} \mathcal{J}_i X_i(\boldsymbol{\sigma}). \tag{14}$$

By assuming that the function $J_0(x)$ is analytic in the interval [0-1], it can be expanded as a power series,

$$J_0(x) = \sum_{k=0}^{k_{\max}} c_k x^k, \tag{15}$$

which, for practical purposes, we truncate to a finite order $k_{\max}$. Combining Eqs. 13, 14, and 15 we can write

$$\begin{aligned} P(\boldsymbol{\sigma}) &= \sum_{j=0} \mathcal{K}_j f_j(\boldsymbol{X}(\boldsymbol{\sigma})) \\ f_j(\boldsymbol{X}) &= X_1^j \text{ for } j = 0, 1, ..., k_{\max}, \\ f_j(\boldsymbol{X}) &= X_{j+1-k_{\max}} \text{ for } j > k_{\max}. \end{aligned} \tag{16}$$

From this, we see that the expansion in Eq. 12 represents a nonlinear cluster expansion (CE) with non-linearities restricted to the 1-point cluster. For all other clusters, the expansion remains linear. Consequently, this model is less general (and more complex to implement) than the nonlinear CE that we propose, which includes all possible monomials up to a certain degree, *i.e.*, terms of the form $X_j^{n_j} X_k^{n_k} X_l^{n_l} \ldots$, with $n_j + n_k + n_l + \cdots \leq k_{\max}$, and thus includes Eq.16 as a special case. As a result, due to the lack of nonlinearities in the 2-point clusters, for example, Eq.12 would struggle to produce sparse models for the Redlich-Kister Gibbs energy, leading to similar convergence issues as in the standard CE. Furthermore, in the case of clathrates, where the kink in the mixing energy is related to a nonlinear change in two-body cluster interactions—as shown in Ref. [5] —this approach would clearly underperform compared to the more flexible nonlinear CE.

### A. Bayesian prior distribution for $J_0(x)$

For the sake of completeness, we derive here the extension of the Bayesian prior distribution of the function $J_0$, presented in Eq.(2) of Ref. [4] for the case of nanoparticles, to solids. To this end, one can carry out a limiting procedure, which consists of considering a supercell of size $N$ and then taking the thermodynamic limit $N \to \infty$. For a supercell of size $N$, the possible number of substituents $n$ is in the range $0, 1, ..., N$, corresponding to the concentrations $x_n = n/N$. Thus, one may write the smoothness assumption of Eq. 2 of Ref. [4] as follows:

$$p(J_0) \propto \prod_{n=0}^{N} \exp\left(-\frac{[J_0(x_n) - J_0(x_{n-1})]^2}{2\sigma_0^2}\right) \tag{17}$$

By defining $dx = 1/N$ and taking the limit $N \to \infty$, one can rigorously show that

$$p(J_0) \propto \exp\left(-\frac{1}{2\tau_0^2} \int_0^1 dx\, J_0'(x)^2\right) \tag{18}$$

where $J_0'(x) = dJ_0(x)/dx$ and $\tau_0$ is a constant. Taking into account the power expansion of $J_0(x)$, after a few steps, the following expression for the prior distribution is obtained:

$$p(J_0) \propto \prod_{j=0}^{k_{\max}} \exp\left(-\frac{(j\mathcal{K}_j)^2}{2\tau_0^2}\right) \tag{19}$$

This could now be used in a Bayesian optimization approach in line with Ref. [4] to find the cluster expansion coefficients $\mathcal{K}_j$, while the hyperparameters $k_{\max}$ and $\tau_0$ could be found by cross validation.

---


[1] Chapter 5 - thermodynamic models for solution and compound phases, in *CALPHAD: Calculation of Phase Diagrams*, Pergamon Materials Series, Vol. 1, edited by N. Saunders and A. Miodownik (Pergamon, 1998) pp. 91–126.

[2] S. Rigamonti, M. Troppenz, M. Kuban, A. Hübner, and C. Draxl, `CELL`: a python package for cluster expansion with a focus on complex alloys (2023), arXiv:2310.18223 [cond-mat.mtrl-sci].

[3] `CELL` documentation, `https://sol.physik.hu-berlin.de/cell`.

[4] T. Mueller, Ab initio determination of structure-property relationships in alloy nanoparticles, Phys. Rev. B **86**, 144201 (2012).

[5] M. Troppenz, S. Rigamonti, and C. Draxl, Predicting ground-state configurations and electronic properties of the thermoelectric clathrates $Ba_8Al_xSi_{46-x}$ and $Sr_8Al_xSi_{46-x}$, Chemistry of Materials **29**, 2414 (2017).
